# Supplementary material for: Dirty Pixels: Towards End-to-End Image Processing and Perception
Source: arXiv:1701.06487 ancillary file (2021-05-08)
Supplement: Supplementary file 1 [file supplement.pdf]

# Supplemental Materials

Steven Diamond  Vincent Sitzmann  Stephen Boyd  Gordon Wetzstein  Felix Heide

## 1 Calibration

In this section we discuss the details of the calibration of our image formation model.

### 1.1 PSF calibration

PSFs (point spread functions) offer a compact description of the aberrations of an optical system. For realistic optical systems, PSFs are spatially varying. In order to perform non-blind deconvolution, the PSF of the optical system has to be calibrated. PSF calibration is done with pictures taken under illumination conditions that ensure that no clipping occurs, so that we consider the unclipped image formation model. Furthermore, we have to take into account the Bayer pattern subsampling when estimating our PSF from raw images. For the purpose of PSF calibration we use the following image formation model:

$$y = S\left(v\left(g\left(i\right)\right) * k\right) + \eta. \tag{1}$$

where $i$ is a target scene, $\eta$ denotes additive noise, and $y$ denotes the observation. Formation of $y$ is a projection of $i$ (i.e., the geometric distortion function of the lens and scene-camera projection) denoted by $g(.)$. It also depends on the optical vignetting function of the imaging system denoted by $v(.)$. In the imaging model (1), $k$ represents the lens PSF, and $*$ denotes the 2D convolution operator. $S(.)$ represents the sampling operator according to Bayer's pattern.

With some modifications on the charts introduced in [Mosleh et al. 2015], we use a chart that includes 0.5 expectation Bernoulli noise patterns and some checkerboard features for the camera-scene alignment shown in Fig. 1(a). A print of this chart is used as our synthetic scene $i$. Its picture is used as the observation $y$ (Fig. 1(b)). Checkerboard corners in the picture of $i$ are used to determine the projection function $g(.)$. We estimate local intensity, which is varying due to lens shading, and use that as a weighting factor in the estimation. Hence, we can form a sharp version of the scene as $u = v\left(g(i)\right)$. Given $n$ observations of the scene $x_1 \ldots x_n$ and their sharp correspondences $u_1 \ldots u_n$, we estimate a PSF $k$ for each channel by finding the solution to

$$\hat{\mathbf{k}} = \arg\max_{\mathbf{k}} \left\| \begin{bmatrix} \mathbf{U}_1 \\ \vdots \\ \mathbf{U}_n \end{bmatrix} \mathbf{k} - \begin{bmatrix} \mathbf{S}^\top \mathbf{y}_1 \\ \vdots \\ \mathbf{S}^\top \mathbf{y}_n \end{bmatrix} \right\|_2^2, \text{ s.t. } \mathbf{k} \geqslant 0 \tag{2}$$

where $\mathbf{y}_j \in \mathbb{R}^{NM/4\times 1}$ and $\mathbf{k} \in \mathbb{R}^{R^2\times 1}$ denote the $N/2 \times M/2$ observation $x_j$ and the $R \times R$ channel PSF $k$ in vector form, respectively. The $N \times M$ sharp correspondence $u_j$ of each observation in a convolution matrix form is denoted by $\mathbf{U}_j \in \mathbb{R}^{NM\times R^2}$. In order to account for the super-resolved version of the PSF, each observation is transformed into the sensor resolution space using $\mathbf{S}^\top$ ($\mathbf{S} \in \mathbb{R}^{NM/4\times NM}$ denotes the sampling matrix form of $S(.)$, and $\top$ denotes the matrix transpose). In our experiments, we use 10 observations (and 10 sharp correspondences), i.e., $n = 10$.

The lens PSF varies spatially in camera space. Therefore, the field-of-view of the camera is divided into non-overlapping blocks and the PSF estimation is carried out for each block individually. Fig. 1(c) shows a set of estimated PSFs for the entire field-of-view of a Nexus 5 camera.

### 1.2 Noise calibration

We consider the Poisson-Gauss noise model which is simple yet accurate for our use cases. We follow the modeling framework of [Foi 2009] in which the image $y$ is given by

$$y = x + s(x)\xi, \quad x = \mathrm{E}(y),\ s(x) = \mathrm{std}(y) \tag{3}$$

$\xi$ is an independent random noise such that,

$$s(x)\xi = \eta_{\mathrm{p}}(x) + \eta_{\mathrm{g}} \tag{4}$$

with $\eta_{\mathrm{p}}(x)$ and $\eta_{\mathrm{g}}$ the Poissonian and Gaussian components of the noise which follow the distributions

$$\eta_{\mathrm{p}}(x) \sim \alpha\mathcal{P}(\alpha^{-1}x)$$
$$\eta_{\mathrm{g}} \sim \mathcal{N}(0, \sigma^2)$$

Following [Foi 2009], the amplification by gain $\theta$ is modeled as a scaling $x = \theta\mathring{x}$, where $\mathring{x}$ is the corresponding clean signal without amplification.

Parameters $\alpha$ and $\sigma$ depend on the hardware and the gain $\theta$,

$$\alpha = \mathring{\alpha}\theta, \quad \sigma^2 = \theta\mathring{\sigma}^2 + \mathring{\sigma}'^2, \tag{5}$$

$\mathring{\sigma}^2 + \mathring{\sigma}'^2$ and $\mathring{\alpha}$ are the variance of the Gaussian noise and the value of $\alpha$ in the case of no amplification. $\mathring{\sigma}^2$ is the variance of the Gaussian noise introduced up to the amplification circuitry and $\mathring{\sigma}'^2$ is the variance of the Gaussian noise introduced thereafter. To estimate the noise parameters, we take calibration pictures of a noise chart (*e.g.* [ISO 2014]) at various gains. The estimation procedure from [Foi 2009] yields $\alpha$ and $\sigma$ for each gain, from which we deduce estimates for $\mathring{\alpha}$, $\mathring{\sigma}$ and $\mathring{\sigma}'$. In our use case we verified that we can assume within a good approximation that the Gaussian noise is created only before and up to the amplification, such that

$$\alpha = \mathring{\alpha}\theta, \quad \sigma = \theta\mathring{\sigma} \tag{6}$$

In the case of a clipped observation the model can be written (see [Foi 2009])

$$\hat{y} = \hat{x} + \hat{s}(\hat{x})\hat{\xi}, \quad \mathrm{E}(\hat{y}) = \hat{x},\ \hat{s}(\hat{x}) = \mathrm{std}(\hat{y}) \tag{7}$$

Fig. 2 shows plots of $s(x)$ and $\hat{s}(\hat{x})$ for the Nexus 6P at various ISO levels. The unit of both x-axis and y-axis of these plots is *digital unit* scaled by the maximal possible value of the sensor. Digital unit is the unit of the raw signal $y$, see [EMV 2016] for more details.

## 2 RBF Memory Usage

A practical obstacle to using the RBF parameterization of the proximal operator is that the gradient with respect to the parameters requires excessive memory to store. In the memory limited environment of a GPU the excessive memory usage is a major issue. If the proximal operator is repeated for multiple iterations of an unrolled optimization algorithm or applied to multiple color channels, the memory demands are amplified even further. Training an unrolled optimization algorithm in conjunction with a high-level network becomes impractical.

We now explain the RBF parameterization in detail and show why the gradient requires excessive memory to store. The RBF parameterization of a univariate function $f$ is given by

$$f(x) = \sum_{i=1}^{q} \pi_i \exp\left(-\frac{\gamma}{2}|x - \mu_i|^2\right), \quad (8)$$

where $\pi \in \mathbf{R}^q$, $\gamma > 0$, and $\mu \in \mathbf{R}^q$. Commonly $\gamma$ and $\mu$ are fixed hyper-parameters, while $\pi$ is a trained variable [Schmidt and Roth 2014; Chen and Pock 2015].

In the RBF parameterization of the proximal operator the function (8) is applied elementwise to a multi-channel image $z \in \mathbf{R}^{m \times n \times p}$. The gradient $\frac{\partial f}{\partial \pi_i}(z)$ is given by

$$\frac{\partial f}{\partial \pi_i}(z) = -\gamma \exp\left(-\frac{\gamma}{2}|z - \mu_i|^2\right)(z - \mu_i),$$

where all operations are computed elementwise. Notice that the gradient has the same dimensions as $z$. The full gradient of $f(z)$ with respect to the RBF parameters $\pi$ has $mnpq$ elements, assuming different $\pi$ are used for different channels.

If $z$ is a 24 channel filter response to a $200 \times 200 \times 3$ image, each RBF function has 50 parameters (i.e., $q = 50$), and values are stored as 32-bit floating point numbers, then the gradient takes over 500 Mb to store. Essentially the input image $z$ is split further into $q$ channels. Operating on 20 images at a time would nearly exhaust the memory of an NVIDIA K80 GPU, just to store the gradient of a single RBF proximal operator. The memory needed to store the gradient of the CNN proximal operator, by contrast, is a small multiple of the size of the multi-channel input $z$.

## 3 L-BFGS Initialization and Parameterization

In this section we discuss the parameterization of the low-level image processing unit and the initialization for L-BFGS pretraining. Recall that we used only 1 layer of unrolled HQS and 3 convolutional layers with 24 channels for the CNN proximal operator. We parameterized $\lambda$ and $\beta^1$ as $\lambda/\beta^1 = \exp(\tau)$ to ensure positivity. We used 24 $5 \times 5$ filters with stride 1 for $C$. We parameterized the filters $c_1, \ldots, c_{24}$ as $c_i = \sum_{j=1}^{24} d_j u_{ij} / \|u_i\|_2$, where $d_1, \ldots, d_{24}$ are the DCT basis of $\mathbf{R}^{5\times5}$ excluding the DC component and $u_1, \ldots, u_{24} \in \mathbf{R}^{24}$. The DCT parameterization ensures the filters are well-scaled and zero-mean. we parameterized $\lambda$ and $\beta^1$ as $\lambda/\beta^1 = \exp(\tau)$, and we used 24 $5 \times 5$ filters with stride 1 for $C$. We kept the color channels separate for the denoising unit but merged them in the CNN proximal operator for the joint deblurring and denoising unit.

For both the denoising and joint denoising and deblurring unit, we initialized L-BFGS with $\tau = \log(.1)$ and $u_i = e_i$ for $i = 1, \ldots, 24$. We initialized the CNN proximal operator with Xavier initialization for the weights and constant initialization to zero for the bias [Glorot and Bengio 2010].

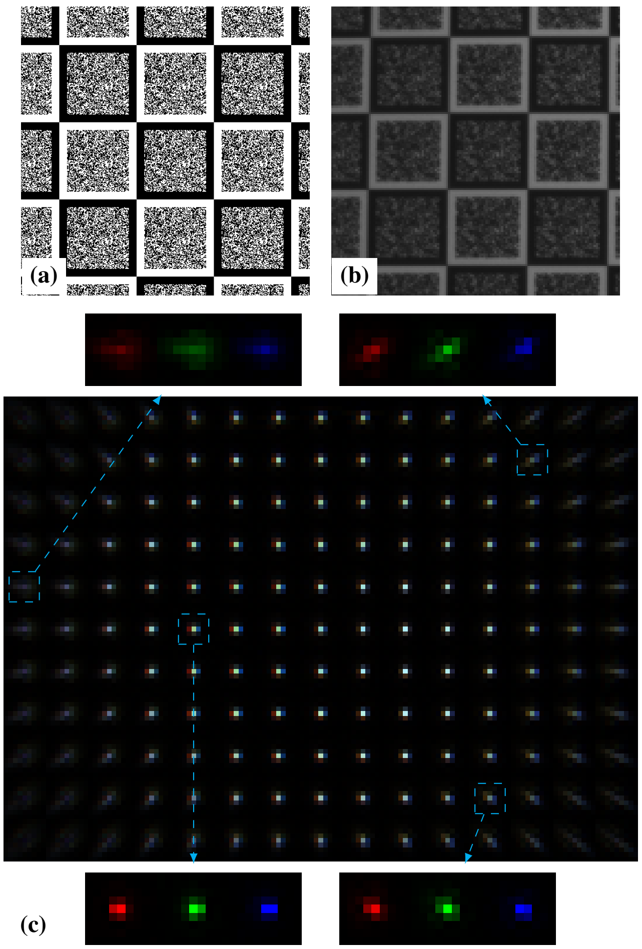


**Figure 1:** *(a) Synthetic pattern (i) used in the PSF estimation. (b) An observation b of the synthetic pattern. (Images in (a) and (b) are scaled to have a similar resolution for a better display here. They have different resolutions in practice.) (c) Lens PSFs measured for a Nexus 5 camera.*

## References

CHEN, Y., AND POCK, T. 2015. Trainable nonlinear reaction diffusion: A flexible framework for fast and effective image restoration. *arXiv preprint arXiv:1508.02848*.

2016. EMVA 1288 Standard for Characterization of Image Sensors and Cameras.

FOI, A. 2009. Clipped noisy images: Heteroskedastic modeling and practical denoising. *Signal Processing 89*, 12, 2609–2629.

GLOROT, X., AND BENGIO, Y. 2010. Understanding the difficulty of training deep feedforward neural networks. In *Aistats*, vol. 9, 249–256.

2014. ISO 12233:2014 Photography – Electronic still picture imaging – Resolution and spatial frequency responses.

MOSLEH, A., GREEN, P., ONZON, E., BEGIN, I., AND PIERRE LANGLOIS, J. 2015. Camera intrinsic blur kernel estimation: A reliable framework. In *The IEEE Conference on Computer Vision and Pattern Recognition (CVPR)*.

SCHMIDT, U., AND ROTH, S. 2014. Shrinkage fields for effective image restoration. In *Proceedings of the IEEE Conference on Computer Vision and Pattern Recognition*, 2774–2781.

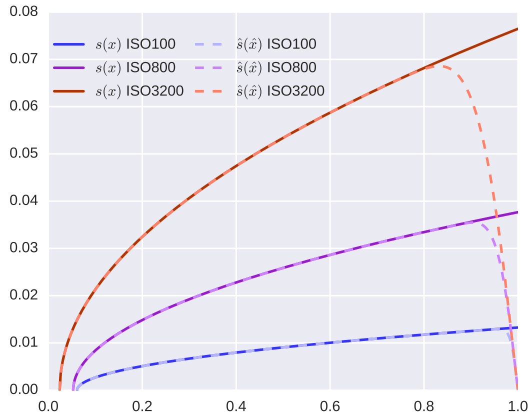


**Figure 2:** $\mathrm{std}(\tilde{y})$ *against* $\mathrm{E}(\tilde{y})$ *and* $\mathrm{std}(y)$ *against* $\mathrm{E}(y)$ *for the Nexus 6P at several ISO levels.*
